# Supplementary material for: Harnessing the Diamond-Air Interface as an Efficient Photon Antenna for Solid-State Emitters
Source: arXiv:2509.26071 ancillary file (2025-09-30)
Supplement: Supplementary file 1 [file Harnessing_the_Diamond_Air_Interface_as_an_Efficient_Photon_Antenna_for_Solid_State_Emitters___Supplementary_Information.pdf]

# Supplementary Information - Harnessing the Diamond-Air Interface as an Efficient Photon Antenna for Solid-State Emitters

Paul Weinbrenner,<sup>†,‡</sup> Aina Lopez Benet,<sup>†</sup> İdil Gözel,<sup>†</sup> and Friedemann

Reinhard<sup>\*,†,‡,¶</sup>

<sup>†</sup>*Institute for Physics, University of Rostock, 18059 Rostock, Germany*

<sup>‡</sup>*Department of Life, Light and Matter, University of Rostock, 18059 Rostock, Germany*

<sup>¶</sup>*Munich Center for Quantum Science and Technology (MCQST), 80799 Munich, Germany*

E-mail: friedemann.reinhard@uni-rostock.de

## Diamond substrate and NV center creation

A IIa-type diamond plate with (100) surface orientation was implanted with  $^{15}\text{N}^+$  ions with an energy of 5 keV and fluence of  $5 \times 10^9$  ions/cm<sup>2</sup>. The depth of the NV centers was estimated from the implantation energy via ion stopping simulations in the work by Pezzagna et al..<sup>1</sup> Annealing of the sample at 830°C for 4 h resulted in an areal NV center density of  $1.0 \mu\text{m}^{-2}$ . The 0.5 mm thick diamond slab was finally polished down to a thickness of 70  $\mu\text{m}$ .

## Optical setup

The microscope objective is an Olympus UPLANSAPO oil immersion objective with 60x magnification and a numerical aperture of 1.35. A 517 nm diode laser was used as excitation light source. Right behind the laser output a polarization filter and  $\lambda/2$ -plate were placed

to enable the polarization-dependent PL measurement in Fig. 2 d and set the polarization to the angle for optimal excitation for each NV center orientation for all other measurements. As tube/Bertrand lens an achromatic doublet with a focal length of 80 mm was used. The monochrome CMOS camera (QHYCCD QHY268M Pro) was mounted on a micrometer stage for moving between the two imaging planes and cooled down to  $-10^{\circ}\text{C}$  for all measurements to reduce dark noise.

## Quantitative comparison of camera and confocal detection

For the quantitative photon rate measurement in the NV center’s image plane we compare the camera measurement with an avalanche photodiode (APD, Excelitas SPCM-AQRH-10) in a confocal microscopy setup with a  $50\text{ }\mu\text{m}$  diameter pinhole. The setup is shown in Fig. 1 a. Both the camera and the pinhole are placed in the focal plane of their respective tube lenses L3 with  $f_3 = 80\text{ mm}$  and L1 with  $f_1 = 150\text{ mm}$ . The pinhole is then imaged onto the APD with lens L2 ( $f_2 = 75\text{ mm}$ ). Importantly for both detection paths the same area of the Airy pattern is integrated over to get the photon rate. This means the region of interest (ROI) on the camera should be equivalent to the pinhole diameter. The different tube lens focal lengths cause a different magnification for each detection path. Taking this into account, the ROI diameter on the camera was determined to be  $50\text{ }\mu\text{m} \times f_3/f_1 \approx 27\text{ }\mu\text{m}$  to image the same area that is transmitted through the pinhole. The photon count rate is measured for multiple NV centers both with and without background subtraction (Fig. 1 b) and shows agreement between the two detection paths, which affirms the validity of the quantitative imaging method.

## Photon detection efficiency and transmission of optical setup

The photon detection efficiency (PDE) and transmission coefficient of the optical setup are calculated by using the manufacturer supplied PDE/transmission data of each detector/optical element in the setup, weighting them with the  $\text{NV}^-$  spectrum<sup>2</sup> and integrating

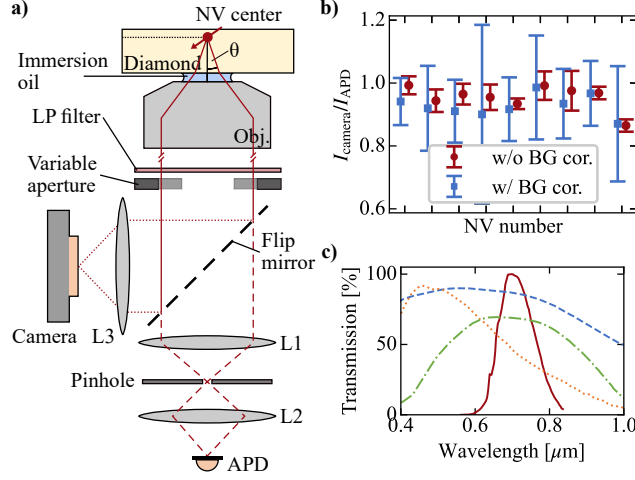

Figure 1: Quantitative comparison of confocal and camera detection. **a)** Experimental setup for comparison of imaging with confocal setup and avalanche photodiode (APD) detection and real-space imaging with a camera. **b)** Ratio between photon count rate measured with camera and confocal setup and APD detection, plotted both with and without background correction. **c)** Spectral dependence of the  $\text{NV}^-$  photoluminescence (red, solid line), the objective transmission (blue, dashed), the camera's quantum efficiency (yellow, dotted) and the APD's photon detection efficiency (green, dash-dotted).

it over the whole spectral range. Fig. 1 c shows the spectral dependence for the components with the most impact on the overall PDE and transmission. The data for all components is summarized in Table 1.

Table 1: Photon detection efficiency and transmission data for the optical setup

| Component                   | Data type    | Value [%] |
|-----------------------------|--------------|-----------|
| Objective                   | Transmission | 85.5      |
| Broadband dielectric mirror | Reflectivity | 99.4      |
| Dichroic mirror             | Transmission | 98.5      |
| Long pass filter            | Transmission | 92.0      |
| Silver coated mirror        | Reflectivity | 98.3      |
| Bertrand/tube lens          | Transmission | 97.2      |
| Camera                      | PDE          | 44.2      |
| Avalanche photo diode       | PDE          | 67.8      |
| Total setup excl. detector  | Transmission | 73.5      |

## Polarization dependent photoluminescence

For the NV centers with different patterns in the BFP image a polarization dependent photoluminescence measurement was performed to support the hypothesis that the different emission patterns originate from the different NV center symmetry axes in the diamond crystal. Two NV centers with BFP images (Fig. 2a and b) rotated by  $90^\circ$  relative to each other are chosen. Fig. 2d shows the normalized count rate of these NV centers as a function of the polarization angle of the excitation light. The photoluminescence curves of the two NV centers are similar but shifted by exactly  $90^\circ$  relative to each other. This means that the NV centers' respective electric dipole configurations, which depend on the NV centers' symmetry axes also differ by a rotation of  $90^\circ$ , when projected onto the (100)-surface plane of the diamond. In Fig. 2h we confirm this with a simulation of the polarization dependent photoluminescence. This calculation also explains the quadruple peak for the curves in Fig. 2d. The total photoluminescence is the sum of emission of the two dipoles. When one dipole approaches saturation of the emission rate (see Eq. 1) the sum of the two curves develops an asymmetry near the maximum intensity.

## Transformation from BFP image to angular emission intensity

Transforming the BFP image coordinates  $(r, \phi)$  to the coordinates of angular emission  $(\theta, \phi)$  with polar angle  $\theta$  and azimuthal angle  $\phi$  requires a non-linear coordinate transformation as well as a correction factor for the intensity. The azimuthal coordinate is identical for the BFP image and the angular emission coordinate system. Light emitted under an angle  $\theta$  will land in the BFP at a radius  $r$ , measured from the center of the BFP image, which is given by  $r(\theta) = r_{90^\circ} \sin \theta$ . The proportionality constant  $r_{90^\circ}$  is found via the knowledge of the value for  $r(0^\circ)$ , i.e. the center of the BFP and  $r(\theta_{NA})$ , where the intensity drops to zero due to the cut-off imposed by the acceptance angle of the objective. The transformation can then be done by inverting the equation above and interpolating the image on the new coordinate grid. Finally, when transforming from the back focal plane to the angular emission intensity

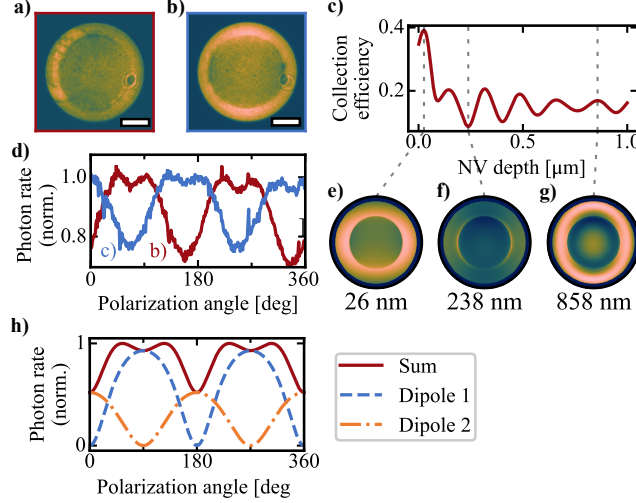

Figure 2: Excitation power and polarization dependence of photon rate. Collection efficiency for varying emitter depth. **a), b)** BFP images of different NV centers. **c)** Photon collection efficiency for back-side detection with normal immersion oil as a function of the NV center depth. The gray, dashed lines indicate the depth for which the BFP images in Fig. 2 e-g were simulated. **d)** Normalized photon rate as a function of the excitation polarization angle for the two NV centers shown in Fig. 2 b and c. **e-g)** Simulated angular emission intensity for different NV depths. The gray, dashed lines indicate the corresponding collection efficiency in c). **h)** Simulation of the polarization dependence of the photoluminescence of a single NV center. The two electric dipole orientations are simulated separately (blue, dashed and yellow, dash-dotted lines respectively) and summed to get the total photon count rate (red, solid line).

the BFP intensity has to be multiplied by the apodization factor<sup>3</sup>  $\cos \theta$ .

## Collection efficiency calculation

The collection efficiency is the ratio of light intensity collected by the objective to the total emitted intensity. For an emitter beneath the surface the latter is calculated by summing two terms. The first is the light intensity that is emitted through the dielectric interface, into the top half-space, taking the Fresnel transmission coefficient at that interface into account. The second term is the intensity emitted into the bottom half of the diamond, which includes the direct downward emission and the reflection from the top surface. For the calculation of the total emitted intensity the last term should not be multiplied with the Fresnel transmission coefficients at the bottom dielectric interface. It should be noted that this total emission

intensity is influenced by the dielectric environment of the emitter and thus depends on its depth beneath the surface. The actually collected intensity for top-side and back-side detection takes both the Fresnel transmission at the respective interfaces as well as the cut-off due to the objectives NA into account. For the case of the NV center under a diamond SIL the emission is modeled as free dipoles inside the diamond without a dielectric antenna effect, because of the large distance between emitter and the top and bottom diamond surfaces. The collected intensity is calculated as the dipoles' emission intensity into the top half-space multiplied with the Fresnel transmission coefficients, for which it is assumed all emitted light impinges onto the diamond-air interface at an incidence angle of  $0^\circ$ . Similar to the collection through a planar diamond surface, a cut-off for a  $NA = 0.95$  objective is applied. The total emission intensity in this case is simply given by the emission of the dipoles integrated over the full solid angle.

## Depth dependence of collection efficiency

Since the dielectric antenna effect strongly depends on the distance between emitter and surface, we investigate how the back-side collection efficiency with immersion oil changes with the depth of the NV center. Fig. 2c shows that there is a decline of the collection efficiency within the first  $\approx 200$  nm and a distinct oscillation with a period of  $\approx 160$  nm. When choosing an implantation depth for deep defect centers this behavior should be taken into account.

Furthermore, the emitter-surface distance drastically changes the emission pattern, as can be seen in Fig. 2e-g. We propose that BFP imaging can be used to determine the NV center's depth as well as its orientation (see main text) in a single measurement.

## Saturation photon rate measurement

The saturation curve  $I_{\text{sat}}$  was first measured in a confocal microscopy setup (see Fig. 1 a) by plotting the photon rate as a function of the excitation power  $P$  as shown in Fig. 3 a and fitting the measurement data to the following equation:

$$I(P) = \frac{I_{\text{sat}}}{1 + \frac{P_{\text{sat}}}{P}} + bP + I_{\text{dark}} . \quad (1)$$

$P_{\text{sat}}$  is the saturation power,  $b$  describes a non-saturating background fluorescence and  $I_{\text{dark}}$  is the detector dark count rate. All further measurements were conducted at an excitation power of 0.6 mW. To convert to the saturation count rate for these measurements the ratio of  $I_{\text{sat}}$  and the count rate at 0.6 mW from the confocal measurement above was determined to be  $1.76 \pm 0.1$ . The unsaturated photon rate was then multiplied by this factor to get the saturation count rate.

## Comparison of back-side and top-side detection

The same NV center from the quantitative photon rate analysis in Fig. 3 in the main text was also imaged from the top-side using the same oil immersion objective as for back-side collection. The resulting real space image is shown in Fig. 3 c and d. Since the depth of the NV center inside the diamond is only  $\approx 8$  nm from this side, the strong spherical aberrations are not visible here. Analyzing the photon rate as a function of ROI diameter in Fig. 3 e also shows that the intensity is focused onto a smaller spot and not spread out by spherical aberrations. While the total intensity inside the  $27 \mu\text{m}$  ROI is larger than for back-side collection, as can be seen in Fig. 3 e and the saturation intensity measurement in Fig. 3 b, the total intensity in the  $1.4 \text{ mm}$  ROI is smaller.

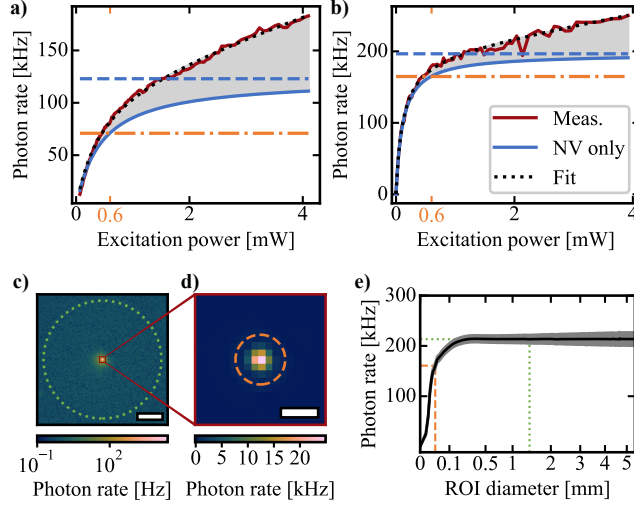

Figure 3: Saturation intensity measurement and top-side collection. **a)** Excitation power dependence of photon rate without background correction. The black, dotted line shows the fit with Eq. 1 to the measurement data (red, solid line). The blue, solid curve shows the NV center’s count rate after subtracting the background and dark count rate from the fitted data. The saturation count rate and intensity at the laser power used for all other measurements (0.6 mW) are indicated by the blue, dashed and yellow, dash-dotted lines respectively. **b)** Saturation intensity measurement for the same NV center as in a), but with top-side, oil-immersion detection. **c)** Emission intensity in NV center image plane using top-side, oil-immersion detection. The color scale is logarithmic for better visibility. The green, dotted outline indicates region of interest (ROI) with 1.4 mm diameter. Scale bar width corresponds to 300  $\mu\text{m}$ . **d)** Zoom into the image in c), but with linear color scale. The circular ROI with yellow, dashed outline shows the edge of the Airy disk with 27  $\mu\text{m}$  diameter. Scale bar width corresponds to 20  $\mu\text{m}$ . **e)** Photon rate within circular ROIs with different diameter in the NV center image plane with the uncertainty illustrated by the shaded region. The yellow, dashed (green, dotted) line marks the photon rate for a 27  $\mu\text{m}$  (1.4 mm) ROI (cf. c and d). The x axis is scaled quadratically.

## References

- (1) Pezzagna, S.; Naydenov, B.; Jelezko, F.; Wrachtrup, J.; Meijer, J. Creation Efficiency of Nitrogen-Vacancy Centres in Diamond. *New J. Phys.* **2010**, *12*, 065017.
- (2) Zhu, X.; Saito, S.; Kemp, A.; Kakuyanagi, K.; Karimoto, S.-i.; Nakano, H.; Munro, W. J.; Tokura, Y.; Everitt, M. S.; Nemoto, K.; Kasu, M.; Mizuochi, N.; Semba, K. Coherent Coupling of a Superconducting Flux Qubit to an Electron Spin Ensemble in Diamond. *Nature* **2011**, *478*, 221–224.



- (3) Richards, B.; Wolf, E. Electromagnetic Diffraction in Optical Systems, II. Structure of the Image Field in an Aplanatic System. *Proceedings of the Royal Society of London. Series A. Mathematical and Physical Sciences* **1997**, *253*, 358–379.
